# Supplementary material for: "Do it my way!": Impact of Customizations on Trust perceptions in Human-Robot Collaboration
Source: arXiv:2310.18791 source file (2023-10-28)
Supplement: Supplementary file 1 [file appendix.tex]

Add link to google forms
Add user interface figure here
Add links to videos here? 
Add meta comments here
